# Supplementary material for: Direct observation of the effects of spin dependent momentum of light in optical tweezers
Source: arXiv:2004.04064 source file (2020-04-08)
Supplement: Supplementary file 1 [file supplementary_material_Spin_momentum.pdf]

# Supplementary Information

**Debapriya Pal**[1], **Subhasish Dutta Gupta**[2,3], **Nirmalya Ghosh**[1,**], **and Ayan Banerjee**[1,*]

[1] *Department of Physical Sciences, Indian Institute of Science Education and Research Kolkata, Mohanpur 741246, India*
[2] *School of Physics, Hyderabad Central University, Hyderabad 500046, India*
[3] *TIFR Centre for Interdisciplinary Sciences, Hyderabad 500107, India*
[*] *Corresponding author: ayan@iiserkol.ac.in*
[**] *Corresponding author: nghosh@iiserkol.ac.in*

*Compiled April 7, 2020*

http://dx.doi.org/10.1364/optica.XX.XXXXXX

## 1. THEORETICAL CALCULATIONS

We use the Debye-Wolf theory[1–4] and angular spectrum representation[5] to determine the exact nature of electric field distribution due to tight focusing of beam inside a stratified medium. Using the angular spectrum method, we decompose the input Gaussian beam (propagating in the z-direction) into plane waves and propagate each wave through the stratified medium while keeping track of the polarization of the wave as it propagates through different stratified media. We then superpose the plane waves at each z position, and recover the beam. The process is then reiterated at every z position of interest. Depolarization results in the beam getting polarized along the direction of propagation(z) even when the incident beam had no longitudinal component of polarization. The relationship between the focused field and incident field is given by a transfer function which incorporates various effects such as depolarization due to tight focusing and the effects of stratification. The transfer function is given by $A = R_z(\phi)TR_y(\theta)R_z(-\phi)$ where $R_z$ and $R_y$ are SO(3) rotation matrices around the respective axis by angle $\phi$, $\theta$ and T is a matrix containing the Fresnel transmission coefficients, $T_s(R_s)$ and $T_p(R_p)$, which include the multiple interface contributions for s and p polarizations respectively introduced by polarization dependence of the field propagating in the stratified medium. The resident field amplitude $\boldsymbol{E_{res}}(\theta,\phi)$ can be written in terms of the incident amplitude $\boldsymbol{E}_{inc}(\theta,\phi)$ as

$$\boldsymbol{E_{res}}(\theta,\phi) = A\boldsymbol{E}_{inc}(\theta,\phi) \tag{S1}$$

This transfer function suggests the plane of the frame is rotated such that the plane of incidence is the xz plane. The depolarization action is effected by the application of $R_y(\theta)$. The effects of interfaces is taken care by T and then the frame is rotated back again to original. For backward propagating waves, the rotation matrix $R_y(\theta)$ is replaced by $\pi$ - $\theta$. The T matrix is replaced by R for the field propagating in the negative direction and given by:

$$T = \begin{pmatrix} T_p & 0 & 0 \\ 0 & T_s & 0 \\ 0 & 0 & T_p \end{pmatrix}; \quad R = \begin{pmatrix} -R_p & 0 & 0 \\ 0 & R_s & 0 \\ 0 & 0 & -R_p \end{pmatrix} \tag{S2}$$

While in general, $\boldsymbol{E_{res}}(\theta,\phi)$ would be a superposition of forward and backward propagating waves in the stratified medium, the dominant contribution would come from the forward propagating waves. The final field is obtained by integrating Eq. (S1) over $\theta$ and $\phi$, so the modified output electric field is give by the form:

$$\boldsymbol{E}(\rho,\psi,z) = i\frac{kfe^{-ikf}}{2\pi}\int_0^{\theta_{\max}}\int_0^{2\pi}\boldsymbol{E}_\infty(\theta,\phi)e^{\pm ikz\cos(\theta)}\times e^{ik\rho\sin(\theta)\cos(\phi-\psi)}\sin(\theta)d\theta d\phi \tag{S3}$$

where r represents f or focal length of the lens. The integration is limited to $\theta_{max}$ because of the finite size of the aperture and decided by the numerical aperture of the microscope objective. Now for input right circular polarized light given by Jones vector $\begin{bmatrix} 1 & i & 0 \end{bmatrix}^T$, the output electric can be written as:

$$\begin{bmatrix} E_x \\ E_y \\ E_z \end{bmatrix} = C\begin{bmatrix} I_0 + I_2\cos 2\psi & I_2\sin 2\psi & 2iI_1\cos\psi \\ I_2\sin 2\psi & I_0 - I_2\cos 2\psi & 2iI_1\sin\psi \\ -2iI_1\cos\psi & -2iI_1\sin\psi & I_0+I_2 \end{bmatrix} \times \begin{bmatrix} 1 \\ i \\ 0 \end{bmatrix} = C\begin{bmatrix} I_0 + I_2\cos 2\psi + iI_2\sin 2\psi \\ I_2\sin 2\psi + i(I_0 - I_2\cos 2\psi) \\ -2iI_1\cos\psi + 2I_1\sin\psi \end{bmatrix} \tag{S4}$$

The transmitted and reflected components of $I_0(\rho)$, $I_1(\rho)$ and $I_2(\rho)$ would be (suffixes t and r imply transmitted and reflected

respectively) given by:

$$I_0^t = \int_0^{\theta_{\max}} E_{inc}(\theta)\sqrt{\cos\theta}\left(T_s^{(1,j)} + T_p^{(1,j)}\cos\theta_j\right) \times J_0\left(k_1\rho\sin\theta\right) e^{ik_j z\cos\theta_j}\sin\theta d\theta$$

$$I_1^t = \int_0^{\theta_{\max}} E_{inc}(\theta)\sqrt{\cos\theta} T_p^{(1,j)}\sin\theta_j \times J_1\left(k_1\rho\sin\theta\right) e^{ik_j z\cos\theta_j}\sin\theta d\theta$$

$$I_2^t = \int_0^{\theta_{\max}} E_{inc}(\theta)\sqrt{\cos\theta}\left(T_s^{(1,j)} - T_p^{(1,j)}\cos\theta_j\right) \times J_2\left(k_1\rho\sin\theta\right) e^{ik_j z\cos\theta_j}\sin\theta d\theta$$

$$I_0^r = \int_0^{\theta_{\max}} E_{inc}(\theta)\sqrt{\cos\theta}\left(R_s^{(1,j)} - R_p^{(1,j)}\cos\theta_j\right) \times J_0\left(k_1\rho\sin\theta\right) e^{ik_j z\cos\theta_j}\sin\theta d\theta$$

$$I_1^r = \int_0^{\theta_{\max}} E_{inc}(\theta)\sqrt{\cos\theta} R_p^{(1,j)}\sin\theta_j \times J_1\left(k_1\rho\sin\theta\right) e^{ik_j z\cos\theta_j}\sin\theta d\theta$$

$$I_2^r = \int_0^{\theta_{\max}} E_{inc}(\theta)\sqrt{\cos\theta}\left(R_s^{(1,j)} + R_p^{(1,j)}\cos\theta_j\right) \times J_2\left(k_1\rho\sin\theta\right) e^{ik_j z\cos\theta_j}\sin\theta d\theta$$

where t and r superscripts denote transmitted and reflected components respectively. We can rewrite output electric field vector from Eq. (S4) as:

$$E_{RCP} = I_0 \begin{bmatrix} 1 \\ i \\ 0 \end{bmatrix} + I_2\exp(i2\psi)\begin{bmatrix} 1 \\ -i \\ 0 \end{bmatrix} - 2iI_1\exp(i\psi)\begin{bmatrix} 0 \\ 0 \\ 1 \end{bmatrix}$$

The first component has the same form as the input field. The second component has helicity of a circularly polarized component with orbital angular momentum l = ±2, respectively, and linearly polarized longitudinal components with topological charge with l = ±1 is generated with input circular polarization having only transverse component. The associated coefficients $I_2(\rho)$ and $I_1(\rho)$ of the transverse (second term) and the longitudinal (third term) field components thereby determine the strength of the spin-orbit angular momentum conversion.

We can similarly calculate the output electric field for left circular polarized light given by input Jones vector given by $\begin{bmatrix} 1 & -i & 0 \end{bmatrix}^T$. We calculate the radial intensity distribution of electric field which is given by:

$$I(\rho) = 2\left|I_0\right|^2 + 2\left|I_2\right|^2 + 4\left|I_1^2\right| \qquad \text{(S5)}$$

Thus, the radial intensity has become $\psi$ independent and the form is same for both left and right circular polarized light. Also intuitively saying, circular polarized system is a symmetric system thus no Spin Hall Shift appears. The intensity of concentric lobes may be enhanced depending on the values of $I_0$, $I_1$, $I_2$ which in turns depend on the stratification.

## 2. NUMERICAL SIMULATIONS

We now run simulations on our experimental system (stratified medium in the path of the optical tweezers light beam) as described in the primary manuscript for circular polarized input light. From Eq. (S5), we calculated the radial intensity of circularly polarized light and observed that there is no $\psi$ dependence. Thus, there are no separate lobes of higher intensity inside the off-axis secondary maxima, as a result of which there is no preferential trapping inside these side lobes. From Fig. S1, we observe there is formation of high intensity rings centered around the z axis. This is easily explained as the circular polarization can be written as the sum of two orthogonal polarizations. Thus, the high intensity lobes due to orthogonal linear polarizations would combine to give high intensity rings. The intensity distribution is same for both matched and mismatched RI cover-slips as shown in Fig. S1a and S1c at focus. We are working with fast diverging Gaussian beam, thus the off-axis intensity in the radial beam profile increases as we move 2$\mu m$ beyond focus as shown in Fig. S1c and S1d. In Fig. S1d, we plot the intensity distribution at z= 2$\mu m$ beyond focus for mismatched 1.814 RI cover-slip, and observe that the off-axis intensity increases, since we introduce larger bending of the incident light by increasing the refractive index contrast.

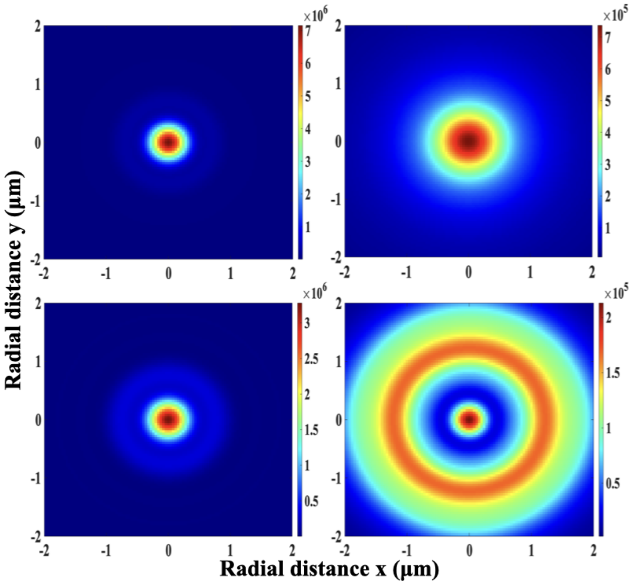


**Fig. S1.** Electric field intensity for coverslips of RI 1.516 at a) focus; b) 2 $\mu m$ beyond focus; coverslips of RI 1.814 at c) focus; d)2 $\mu m$ beyond focus

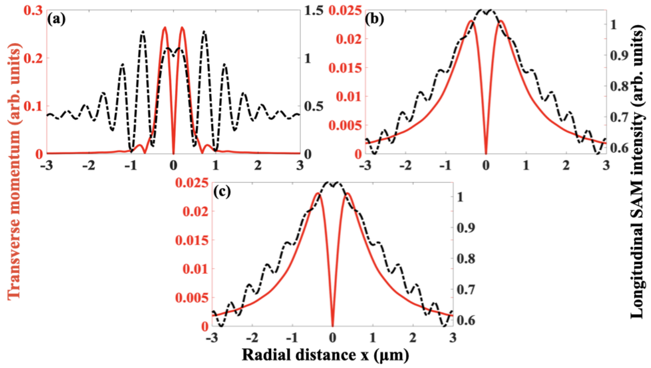


**Fig. S2.** Longitudinal Spin Angular Momentum Intensity(black) and transverse spin momentum (red) plot for coverslip of RI 1.516 at a) focus; (b) 1 $\mu m$;and c) 2 $\mu m$ away from focus

We plot Fig. S2 for the matched condition at different axial planes. We observe that the LSAM - depicted by black lines - is always high at the beam center, where the intensity is also maximum.

## 3. EXPERIMENT

### A. Sample preparation

As discussed in primary manuscript, we have used RM257 vaterite liquid crystal particle, which are optically anisotropic and therefore birefringent in nature - as the probe particle for our experiment to observe the rotation dynamics and spin momentum locking effects. Understandably, these are birefringent particles, which can exchange angular momentum with the input light. We have synthesized RM257 vaterite particle using the following procedure:

- We use two hot plates with temperature sensors.
- We take 150 ml of de-ionized water and 50 ml ethanol and heat them to 75 and 50 degrees, respectively.
- We add 30 mg of RM257 to the ethanol when it reaches 55 degrees and wait till the solution gets clear again.
- Once water reaches 70 degrees we add the ethanol dropwise to it, making sure that we cover the mouth of the beaker which contains ethanol to reduce the evaporation rate of the latter. The slowly we add the liquid, the bigger will be the particles.
- Thus, the more time one spends to make the ethanol evaporate, the bigger the size of the RM257 particles. We cover the mixture beaker with aluminium foil while heating and make some holes to reduce the evaporation rate. Once all the ethanol is evaporated, we switch off the hot plates, and allow the solution to cool.

### B. Verification of birefringence

In order to verify the birefringence characteristics of the particles (which are also non-spherical), we take it in an aqueous dispersion in the sample chamber, expose it to the tweezers laser, and rotate the $\lambda/4$ plate at the input end of our setup, and observe the intensity of the particle w.r.t the background. If the particle is birefringent, then the intensity of particle will change with the rotation of the $\lambda/4$ plate. We observe the same and thus verify the birefringence property of the particle.

### C. Determination of frequency of rotation of probe particles

From the videos provided in the Supplementary Information - we evaluate the trajectories of the particles as a function of time using the software ImageJ by tracking the centroid of the particle. The trajectory thus consists of the rotation which is modulated by the inherent Brownian motion of the particle. Then, we determine the power spectral density (PSD) of the particle displacement, which gives peaks at the different rotation frequencies corresponding to different power levels. We also divide the motion into different time bins corresponding to the the different laser powers and evaluate the PSD at each bin to find out the particular frequency of rotation at a given power level.

## 4. MEDIA

Videos 1 and 2 depict rotation of different birefringent particles for right and left circularly polarized Gaussian beams, respectively. Video 3 depicts the rotation of the same particle when the polarization is changed during the experiment. We first observe rotation around the beam axis for input RCP, which changes to rotation around the particle axis for input LCP. Videos 4 - 7 depict increase in rotation frequency of particles with increase in laser power.

## REFERENCES


1. M. Born and E. Wolf, "Principles of optics, corregida," (1989).
2. E. Wolf, "Electromagnetic diffraction in optical systems-i. an integral representation of the image field," Proc. Royal Soc. Lond. Ser. A. Math. Phys. Sci. **253**, 349–357 (1959).
3. B. Richards and E. Wolf, "Electromagnetic diffraction in optical systems, ii. structure of the image field in an aplanatic system," Proc. Royal Soc. Lond. Ser. A. Math. Phys. Sci. **253**, 358–379 (1959).
4. K. Y. Bliokh, E. A. Ostrovskaya, M. A. Alonso, O. G. Rodríguez-Herrera, D. Lara, and C. Dainty, "Spin-to-orbital angular momentum conversion in focusing, scattering, and imaging systems," Opt. express **19**, 26132–26149 (2011).
5. L. Novotny and B. Hecht, *Principles of nano-optics* (Cambridge university press, 2012).
